# Supplementary material for: Deep representation learning for human motion prediction and classification
Source: arXiv:1702.07486 source file (2017-04-13)
Supplement: Supplementary file 1 [file appendix.tex]

\section*{A. Appendix}
\label{sec:appendix}

In this section, we give a detailed account of the implementation and training procedure of the models. 

\subsection*{A.1 Detailed model structure}

The input and output data for all models is of dimension $3 \ \x \ N_{joints}  \ \x \ \Delta t = 3 \ \x \ 24 \ \x \ 100$. While these dimensions are retained for the input layer, the output layer is flattened to 7200 dimensions. The weights of all layers are initialized sparsely and with a Gaussian distribution (mean = 0, variance = 1). We apply a sigmoid non-linearity to all layers except the bottleneck layer, the output layer of the temporal encoders and the output layer of the classifiers. We do not apply any pooling. Instead of eliminating information by pooling or by applying a rectified linear non-linearity, it has proven to be crucial to let all information flow freely from the input to output layer.  

We denote the dimension of a fully-connected layer by a single number of output dimensions D and the connection between layer D and E by D--E. Layers can be parallel in a network, i.e. they are all connected to parts of the same input and output layer but not to each other. When the neighbouring layers have the same structure Q, we denote this by {Q$i$}$_{j = 1:M}$, where M is the number of such layers. Furthermore, we denote the number of output neurons N and the filter size of a convolutional layer by [N,$\Delta t^w$].

All layers of the symmetric temporal encoder are fully-connected. The structure of the network is depicted in Figure \ref{fig:netsstruc} a).

A number of layers in the convolutional encoder are convolutional with a filter of size $3 \ \x \ N_{joints}  \ \x \ \Delta t^w$.   The structure of the convolutional encoder is depicted in Figure \ref{fig:netsstruc} b).

Finally,  the hierarchical temporal encoder contains 24 parallel layers in the first level of the hierarchy representing a single joint dimension in the data layer. The second layer combines these nodes into separate limbs. In the following, the arms and legs are summarized in a node each and form the body together with the trunk in the subsequent layer. This network is depicted in Figure \ref{fig:netsstruc} c).

The structure of the classifier for input data with dimension N and M classes is N--50--20--M, where the last layer is a softmax layer.

\begin{figure}[t]
\begin{center}
   \includegraphics[width=0.8\linewidth]{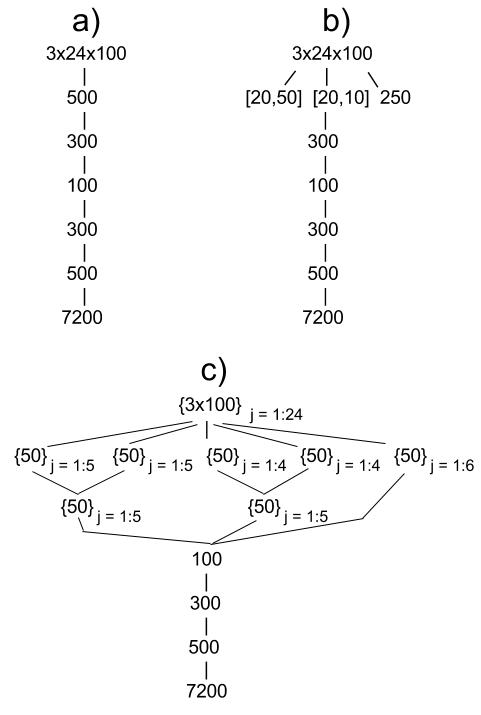}
\end{center}
   \caption{The structure of the symmetrical temporal encoder (a)), the convolutional temporal encoder(b)) and the hierarchical temporal encoder (c))}
\label{fig:netsstruc}
\end{figure}

\subsection*{A.2 Training details}

We implement and train our models  with help of the Caffe deep learning framework  \cite{jia2014caffe}. For this, we shuffle the training and testing data randomly, making sure that the temporal structure between data points of the same recording disappears. We train mini-batches of 300 to 500 data points with a learning rate of 0.01, a weight decay of 0.0005 and momentum of 0.9. We apply an increasing amount of dropout on the input data layer, ranging from 0.1 to 0.3.
